# Supplementary material for: N-Modal Contrastive Losses with Applications to Social Media Data in Trimodal Space
Source: arXiv:2403.12747 source file (2024-03-18)
Supplement: Supplementary file 1 [file supp_mat.tex]

\begin{figure}[t!]
\includegraphics[width=1.96\linewidth]{Figures/qualitative_whole.pdf} % Reduce the figure size so that it is slightly narrower than the column.
\vspace{-2mm}
\caption{The qualitative results with the original, untranslated captions that were posted with the image. Google translate was used for the translation, so slight inconsistencies may exist. Hence the need to include captions in the original.}
\vspace{-2mm}
\label{fig:quali}
\end{figure}

%\end{document}
